# Supplementary material for: PtyRAD: A High-performance and Flexible Ptychographic Reconstruction Framework with Automatic Differentiation
Source: arXiv:2505.07814 source file (2025-07-11)
Supplement: Supplementary file 1 [file SI.pdf]

# Supplementary Information

# PtyRAD: A High-performance and Flexible Ptychographic Reconstruction Framework with Automatic Differentiation

Chia-Hao Lee,[*,†] Steven E. Zeltmann,[‡] Dasol Yoon,[¶] Desheng Ma,[†] and David A. Muller[*,†,§]

†*School of Applied and Engineering Physics, Cornell University, Ithaca, New York 14850, United States*

‡*Platform for the Accelerated Realization, Analysis, and Discovery of Interface Materials, Cornell University, Ithaca, New York 14850, United States*

¶*Department of Materials Science and Engineering, Cornell University, Ithaca, New York 14850, United States*

§*Kavli Institute at Cornell for Nanoscale Science, Cornell University, Ithaca, New York 14850, United States*

E-mail: chia-hao.lee@cornell.edu; david.a.muller@cornell.edu

# Benchmarking Details

## Hardware and OS Specifications

All benchmarking was performed on a private cluster hosted by the Cornell University Center for Advanced Computing (CAC). The cluster consists of a head node running OpenHPC 2.3 with Rocky Linux 8.4. Computations were carried out on four identical compute nodes, each equipped with dual 64-core AMD EPYC 7713 processors (with hyperthreading enabled, yielding 256 logical CPUs), 1TB of RAM, and four NVIDIA A100 (80 GB) GPUs.

For each reconstruction task shown in Figure 3, all ptychographic reconstruction packages were benchmarked using the same hardware configuration to ensure a fair comparison. Specifically, each job was assigned a 20 GB MIG (Multi-Instance GPU) slice of an NVIDIA A100 80 GB GPU and four CPU cores. MIG is a feature of NVIDIA Ampere GPUs that partitions a single physical GPU into multiple isolated instances, each with dedicated compute cores and memory, allowing multiple jobs to run concurrently without interference. A 20 GB MIG slice corresponds to approximately 2/7 (or 28.6%) of the total GPU memory bandwidth and streaming multiprocessors (SMs) of the full A100 GPU. The number of CPU cores and total CPU memory had negligible impact on the reconstruction time, as all packages fully load the diffraction patterns into GPU memory at the start of computation. Resource allocation, including memory management, was handled automatically by the Slurm job scheduler.

## Software Version and Environments

- **PtyRAD** was run using Python 3.11.9, with PyTorch 2.1.2 and CUDA 11.8. The full Python environment specification is provided in our GitHub repository https://github.com/chiahao3/ptyrad.
- **py4DSTEM** was benchmarked using version 0.14.18,[1] specifically the `baf9e30` com-

mit from the original "`dev`" branch. The environment was built with Python 3.11.10, CuPy 13.3.0, and CUDA 11.8. We introduced several lightweight modifications to the package—such as results saving, timing utilities, and wrapper functions—to facilitate systematic reconstruction from input files. These changes do not modify the core algorithms or affect performance timing. Our modified version is openly available at https://github.com/chiahao3/py4DSTEM/tree/benchmark, and an installation guide is included.

- **PtychoShelves** was tested using the `fold_slice` fork,[2] specifically the `d9a1204` commit from the original "`main`" branch, executed with MATLAB 2021a.

## Package configurations

While all reconstructions in Figures 3 and 4 use the same physical model complexity (e.g., number of object slices, probe modes) and batch sizes across packages, each software package implements its own optimization algorithms and regularization strategies. We summarize the most relevant settings below. Full parameter files for each reconstruction are provided in our Zenodo record for full transparency and reproducibility.

- **PtyRAD**: Uses the Adam optimizer with optimizable parameters including the object amplitude and phase, probe, and probe positions. The base learning rate is set to $5 \times 10^{-4}$, with a separate learning rate of $1 \times 10^{-4}$ for the probe. The loss function includes a normalized root-mean-square error (NRMSE) under a Gaussian noise model, along with an L1 sparsity regularization term weighted by 0.1. Additional regularization techniques include the probe mode orthogonalization, a real-space $r_z$ filter with $\sigma_z = 1$ for multislice reconstruction, positivity constraint for object phase, and a thresholding within [0.98, 1.02] for the object amplitude.

- **PtychoShelves**: Configured with the `GPU_MS` engine using the LSQML algorithm and the `MLs` option, which corresponds to an L1 likelihood model consistent with

the Gaussian noise assumption. The multislice regularization weight $\beta$ is set to 0.1. Optimizable parameters include the complex object, probe, and probe positions. No variable probe is used in these reconstructions.

- **py4DSTEM**: Uses the "gradient descent" solver with default update step size of 0.5. Although we find that setting the step size to 0.1 significantly improves numerical stability. Optimizable parameters include the complex object, probe, and probe positions. The multislice regularization parameter $\beta$ is also set to 0.1, implemented as the `kz_regularization_gamma` parameter. Note that the multislice $k_z$ filters are implemented differently across packages so the regularization strength may not be directly comparable.

Supplementary Table S1: Publicly available ptychography software packages.

| Year | Reference | Supported Algorithms | Language | Notes |
|---|---|---|---|---|
| 2015 | (py)ptychoSTEM[3–5] | SSB,WDD | MATLAB, Python | Direct ptychographic phase reconstructions with 4D STEM data. |
| 2016 | PtyPy[6] | DM, RAAR, ePIE, ML | Python | Support of on-the-fly reconstructions (data being acquired); mixed probe and object |
| 2018 | NSLS-II (Ptycho_gui) [7] | DM | Python | Deployed on NSLS-II beamline machines with GUI |
| 2019 | ptychoSampling [8] | AD | Python | Generalized forward models: near-field ptychography and 3D Bragg projection ptychography |
| 2020 | PtychoShelves[9] | ePIE, DM, LSQML | MATLAB | MATLAB-based GPU-accelerated engine |
| 2020 | PyNX [10] | ER, RAAR, DM, ML | Python | CDI, ptychography, wavefront propagation, scattering calculations, etc. |
| 2020 | abTEM[11] | PIE | Python | A flexible package for simulating TEM experiments |
| 2021 | PtychoNN [12] | Neural Network-based | Python | Predicts sample amplitude and phase from input diffraction data alone |
| 2021 | Ptychopy[13] | ePIE, DM, LSQML | Python | CUDA C++ backend |
| 2021 | py4DSTEM[1] | SSB, WDD, DM, RAAR, GD | Python | A complete toolbox for 4D-STEM data processing beyond ptychography |
| 2021 | Ptychography 4.0 [14] | SSB | Python | Support of live processing of data (SSB method) |
| 2021 | Adorym[15] | AD | Python | HPC AD package for 2D/3D ptychography, CDI, holography, and tomography |
| 2021 | PtychoKeras[16] | AD | Python | AD-based using TensorFlow and Keras |
| 2022 | Tike[17] | ePIE, LSQML | Python | Laminography, tomography from ptychographic reconstructions |
| 2022 | SciComPty[18] | AD | Python | A modular framework for the design of new ptychography algorithms with simulations |
| 2022 | Airpi[19] | Pretrained NN | Python | CNN recovered complex electron wave function from CBEDs |
| 2023 | Deep-CDI[20] | Pretrained NN | Python | CNN predicted convergent diffraction imaging (CDI) |
| 2023 | PtyLab[21] | ePIE family | MATLAB, Python, Julia | Fourier and conventional ptychography; variants of ePIE: mPIE, zPIE, aPIE, pcPIE, e3PIE |
| 2024 | torchslice[22] | AD, | Python | Optimize discrete atomic models to incorporate thermal diffuse scattering |
| 2024 | PtychoFormer [23] | Pretrained NN | Python | Predicts and stitches local patches from sparse scans with optional integration of ePIE |

ML: Maximum Likelihood
WDD: Wigner Distribution Deconvolution
SSB: Single Side Band
DM: Difference Map
ePIE: extended Ptychographical Iterative Engine
ER: Error Reduction
LSQML: Least-Squares Maximum-Likelihood
RAAR: Relaxed-Averaged Alternating Reflections
GD: Gradient Descent
AD: Automatic Differentiation
NN: Neural Network

Supplementary Table S2: Acquisition and reconstruction parameters for each experimental dataset used in Figure 2.

| **Dataset** | **MOSS-6** [24] | **ZSM-5** [25] | **tBL-$WSe_2$** [26] | **$PrScO_3$** [27] |
|---|---|---|---|---|
| Acceleration voltage (kV) | 300 | 300 | 80 | 300 |
| Convergence angle (mrad) | 10 | 15 | 24.9 | 21.4 |
| Defocus (Å)[a] | 885 | 350 | 0 | 0 |
| Real space px size (Å) | 0.2962 | 0.3591 | 0.1494 | 0.0934 |
| Scan pattern | 256×256 | 256×256 | 128×128 | 64×64[b] |
| Scan step size (Å) | 1.051 | 0.3989 | 0.429 | 0.41 |
| Collection angle (mrad) | 33.2 | 27.4 | 139.7 | 105.1 |
| $k_{\mathrm{max}}$ (Å$^{-1}$) | 1.69 | 1.39 | 3.35 | 5.35 |
| Detector pixel | 128 | 128 | 128 | 256[c] |
| Dose ($e^-$/Å$^2$) | 100 | 3500 | 7.55E+05 | 1.22E+06 |
| Slice thickness (Å) | 40 | 40 | 2 | 10 |
| Number of slices | 5 | 8 | 6 | 21 |
| Probe modes | 2 | 6 | 6 | 8 |
| Batch size | 512 | 32 | 32 | 32 |
| Iteration | 20 | 2000 | 4000 | 4000 |

[a] Positive defocus corresponds to underfocus condition.
[b] The available dataset includes only a subset of scan positions used in Chen et al. [27].
[c] Diffraction patterns were padded from 128 to 256 pixels; the available dataset was already zero-padded.

Supplementary Table S3: Parameters for the simulated tBL-$WSe_2$ dataset used in Figure 3a

| **Dataset** | **Simulated tBL-$WSe_2$** |
|---|---|
| Package | abTEM[11] |
| Version | 1.0.6 (pypi) |
| Interlayer twist (°) | 3 |
| Se vacancy density (%) | 2 |
| Supercell size (x, y, z) (Å) | (85.72, 85.66, 14.75) |
| Potential shape (x, y, z) (px) | (861, 861, 15) |
| Real space px size (Å) | 0.0996[a] |
| Slice thickness (Å) | 1 |
| Frozen phonon configurations | 25 |
| Phonon perturbation std. (Å) | 0.1 |
| Acceleration voltage (kV) | 80 |
| Convergence angle (mrad) | 24.9 |
| Defocus (Å) | 0 |
| $C_3$ (nm) | 500 |
| $C_c$ (nm) | 1000 |
| Energy spread std. (eV) | 0.35 [b] |
| Focal spread std. (Å) | 43.75 |
| Number of defoci | 5 |
| Source size std. (Å) | 0.34 [c] |
| Scan pattern | 128×128 |
| Scan step size (Å) | 0.429 |
| Collection angle (mrad) | 139.7 [d] |
| $k_{\mathrm{max}}$ ($Å^{-1}$) | 3.35 [d] |
| Simulated CBED size (px) | 574×574 |
| Final CBED size (px) | 128×128 [e] |
| Dose ($e^-/Å^2$) | 1.0E+06 |

[a] abTEM crops the diffraction pattern to 2/3 $k_{\mathrm{max}}$ for antialiasing at the end so the final pixel size is $0.0996 \times 1.5 = 0.1494$.
[b] Equivalent to an energy spread FWHM of 0.82 eV.
[c] Equivalent to a source size FWHM of 0.80 Å.
[d] Both collection angle and $k_{\mathrm{max}}$ show the final value after antialiasing cropping.
[e] The diffraction patterns are resampled to match the k-space sampling of the experimental dataset.

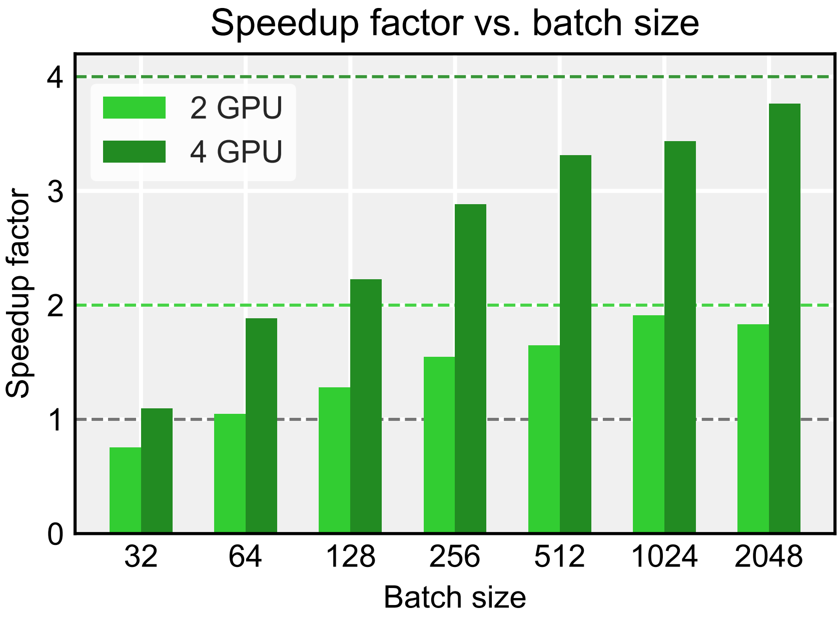


Supplementary Figure S1: Speedup factors for PtyRAD reconstructions on the tBL-$WSe_2$ dataset using 2 and 4 NVIDIA A100 GPUs with varying batch sizes, normalized to single GPU performance. The dashed lines represent the ideal linear speedup for 2 and 4 GPUs. Performance scales sub-linearly with increasing GPU count, particularly for smaller batch sizes, where overhead and inter-GPU communication reduce speedup and may even cause slowdowns.

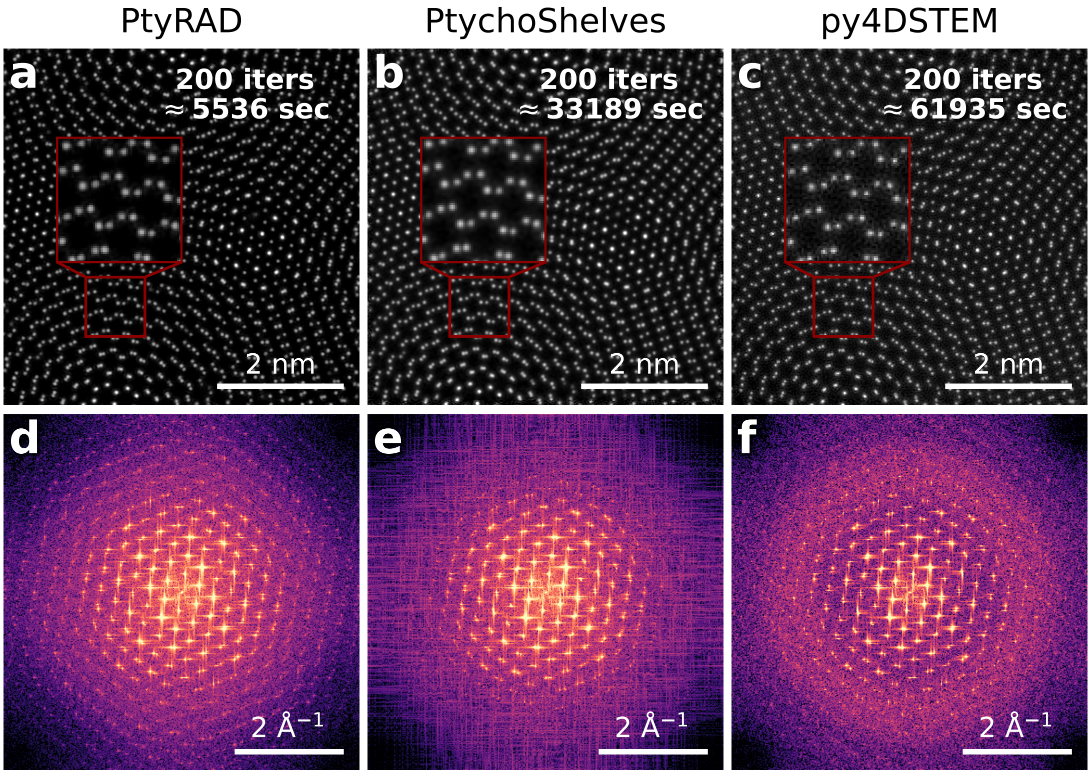


Supplementary Figure S2: Reconstructed phase images of the simulated twisted bilayer $WSe_2$ dataset after 200 iterations using (a) PtyRAD, (b) PtychoShelves, and (c) py4DSTEM and zoom-in insets. (d–f) Corresponding fast Fourier transform (FFT) power spectra of (a–c). Total reconstruction times taken for 12 probe modes, 6 object slices, batch size 16, and 200 iterations are labeled in the top right corners of each panel. All the reconstructions are conducted using the same hardware (a 20 GB MIG slice from a 80 GB NVIDIA A100). PtyRAD achieves higher information transfer given the same number of iterations and a shorter reconstruction time.

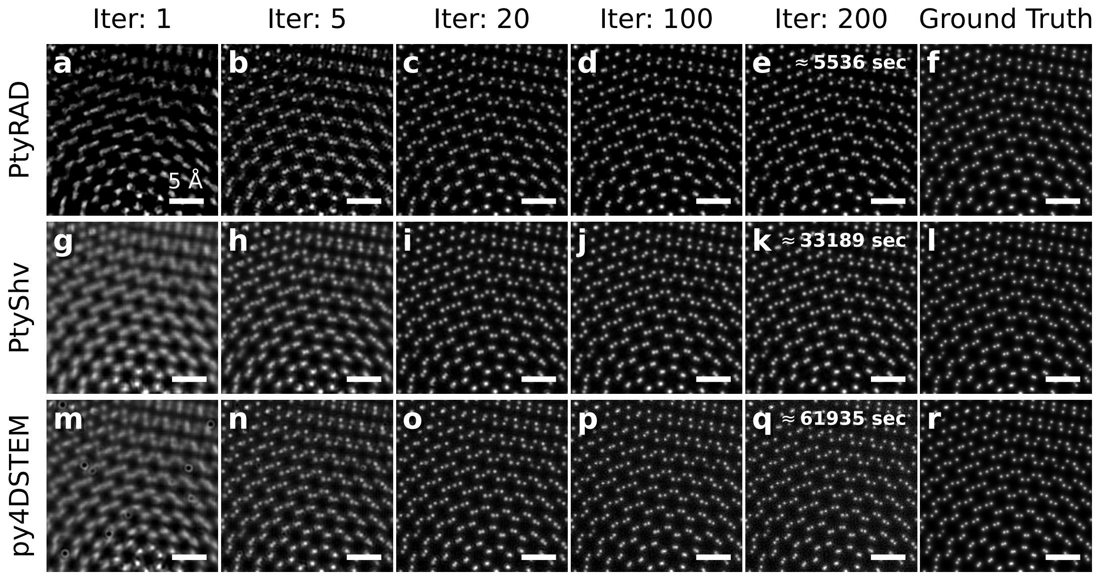


Supplementary Figure S3: Convergence comparison of different ptychographic reconstruction packages: PtyRAD (a–e), PtychoShelves (labeled as "PtyShv", g–k), and py4DSTEM (m–q). The benchmark was conducted on the simulated tBL-$WSe_2$ dataset using the same hardware (a 20 GB MIG slice from a 80 GB NVIDIA A100) with 12 probe modes, 6 object slices, and a batch size of 16 for all packages. Reconstructions are shown at selected iterations (1, 5, 20, 100, and 200) to illustrate the progression toward convergence. The total reconstruction time for 200 iterations (excluding initialization and result-saving time) is indicated in the corresponding column. The ground truth images (f, l, r) are shown in the last column for comparison. PtyRAD completes 200 iterations significantly faster than PtychoShelves and py4DSTEM given the tested condition, achieving a 6× to 11× speedup without compromising reconstruction quality. Scale bars are consistent across all panels.

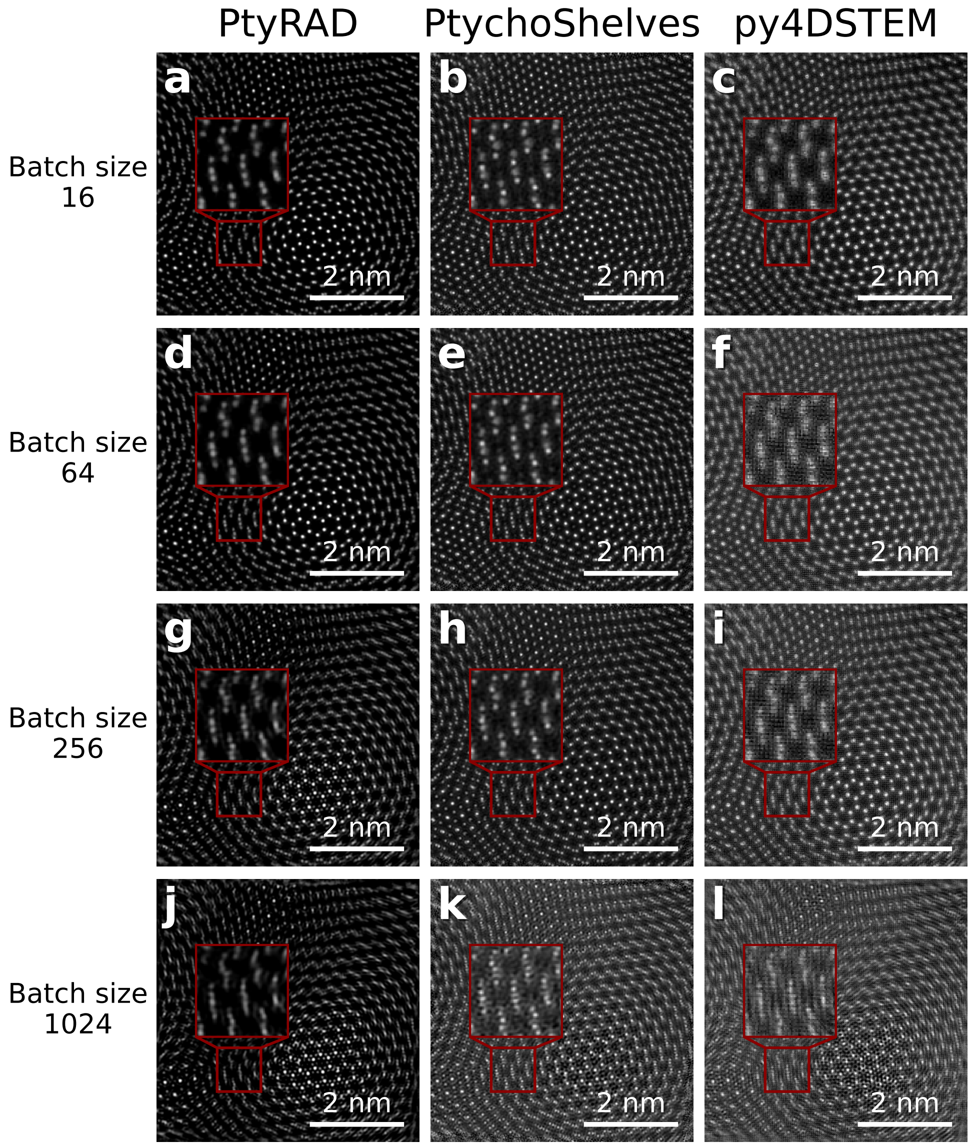


Supplementary Figure S4: Influence of batch size on reconstruction quality. Columns correspond to different reconstruction packages, including PtyRAD, PtychoShelves, and py4DSTEM, respectively. Rows correspond to batch sizes of (a–c) 16, (d–f) 64, (g–i) 256, and (j–l) 1024. All the reconstructions are done on the experimental tBL-$WSe_2$ dataset with 128 by 128 diffraction patterns using 6 probe modes, 6 object slices, and 100 iterations. Insets highlight a magnified region to facilitate visual comparison of structural details. Smaller batch sizes (e.g., 16 and 64) generally yield sharper and more detailed reconstructions compared to larger batch sizes, which exhibit blurring and loss of contrast. Note that PtychoShelves gives stronger but incorrect inter-atomic contrasts for these reconstructions, likely due to the excessive $k_z$ regularization.

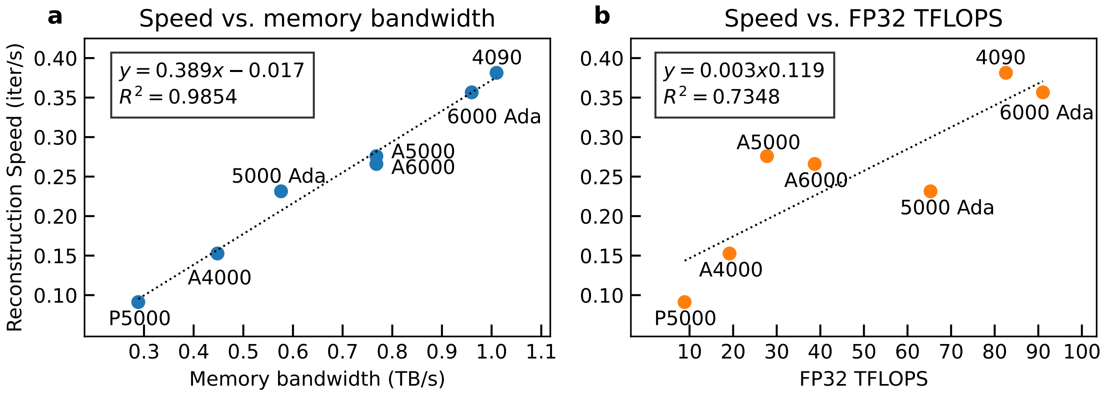


Supplementary Figure S5: Comparison of different GPUs for reconstruction speed using PtyRAD. Reconstruction speed (iterations per second) for PtyRAD is tested on the experimental tBL-$WSe_2$ dataset with 1 slice, 12 probes, and batch size of 256, plotted against (a) the memory bandwidth and (b) the floating point 32 TFLOPS of various NVIDIA GPUs rented via vast.ai. The GPUs tested include P5000, A4000, A5000, A6000, 5000 Ada, 6000 Ada, and 4090. We observe a strong linear correlation ($R^2 = 0.9854$) between GPU memory bandwidth and reconstruction speed, suggesting that PtyRAD is more memory-bandwidth bound than compute-bound.

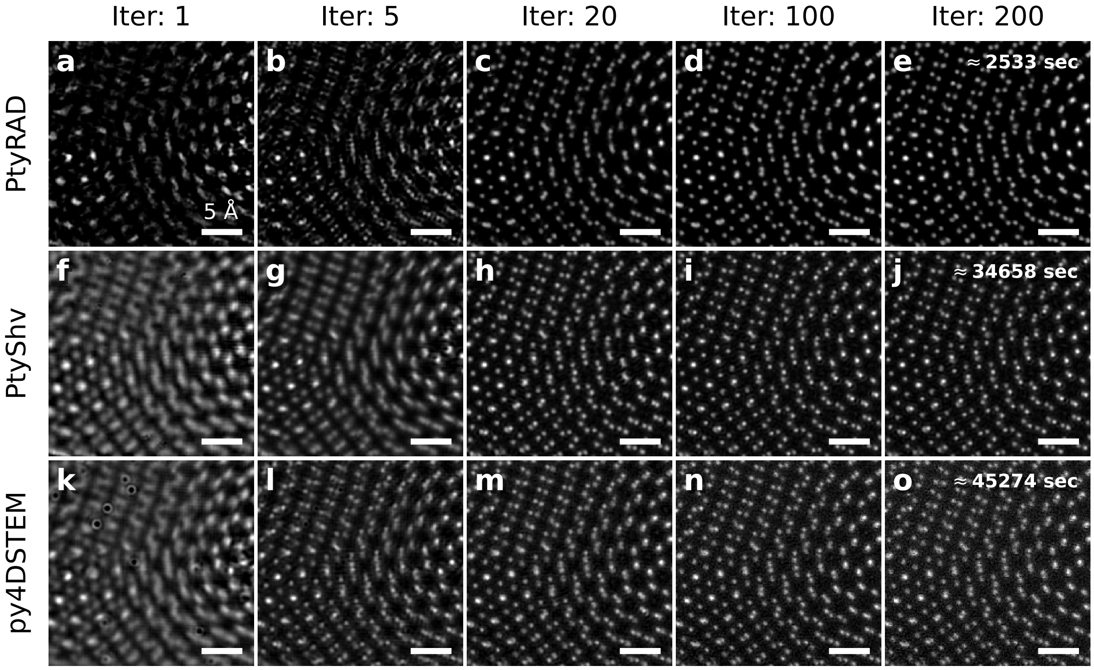


Supplementary Figure S6: Convergence comparison of different ptychographic reconstruction packages: PtyRAD (a–e), PtychoShelves (labeled as "PtyShv", f–j), and py4DSTEM (k–o). The benchmark was conducted on the experimental tBL-$WSe_2$ dataset using the same hardware (a full 80 GB NVIDIA A100) with 12 probe modes, 6 object slices, and a batch size of 16 for all packages. Reconstructions are shown at selected iterations (1, 5, 20, 100, and 200) to illustrate the progression toward convergence. The total reconstruction time for 200 iterations (excluding initialization and result-saving time) is indicated in the last column. PtyRAD completes 200 iterations significantly faster than PtychoShelves and py4DSTEM given the tested condition, achieving a 14× to 18× speedup without compromising reconstruction quality. Scale bars are consistent across all panels.

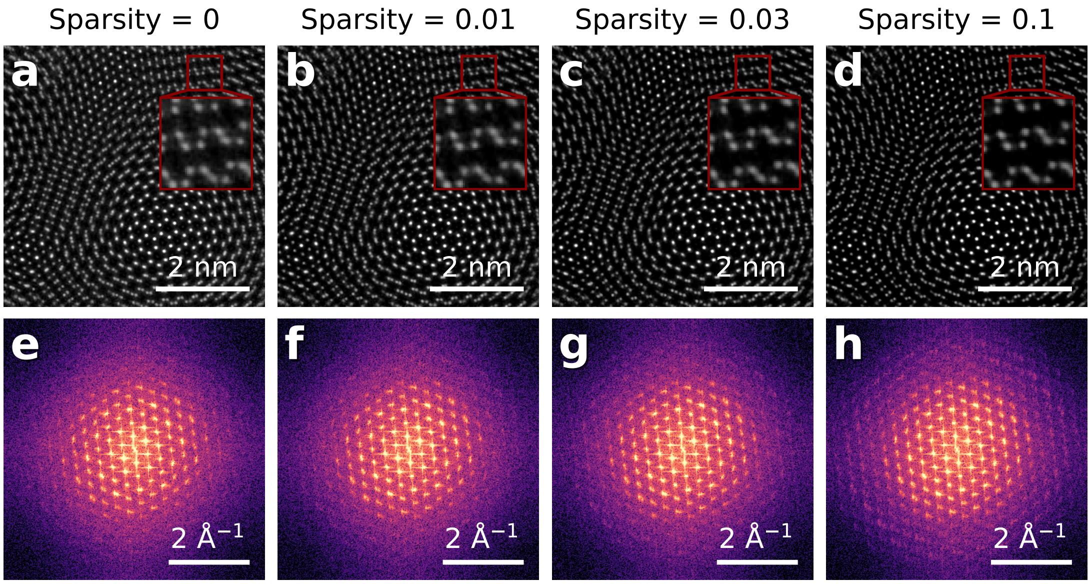


Supplementary Figure S7: Effect of sparsity regularization on ptychographic reconstruction of tBL-$WSe_2$. (a–d) Reconstructed phase images with increasing sparsity regularization weights of 0, 0.01, 0.03, and 0.1, respectively. Red insets show magnified regions highlighting visual details. (e–h) Corresponding FFT power spectra showing the reciprocal space information transfer increase with stronger sparsity regularization.

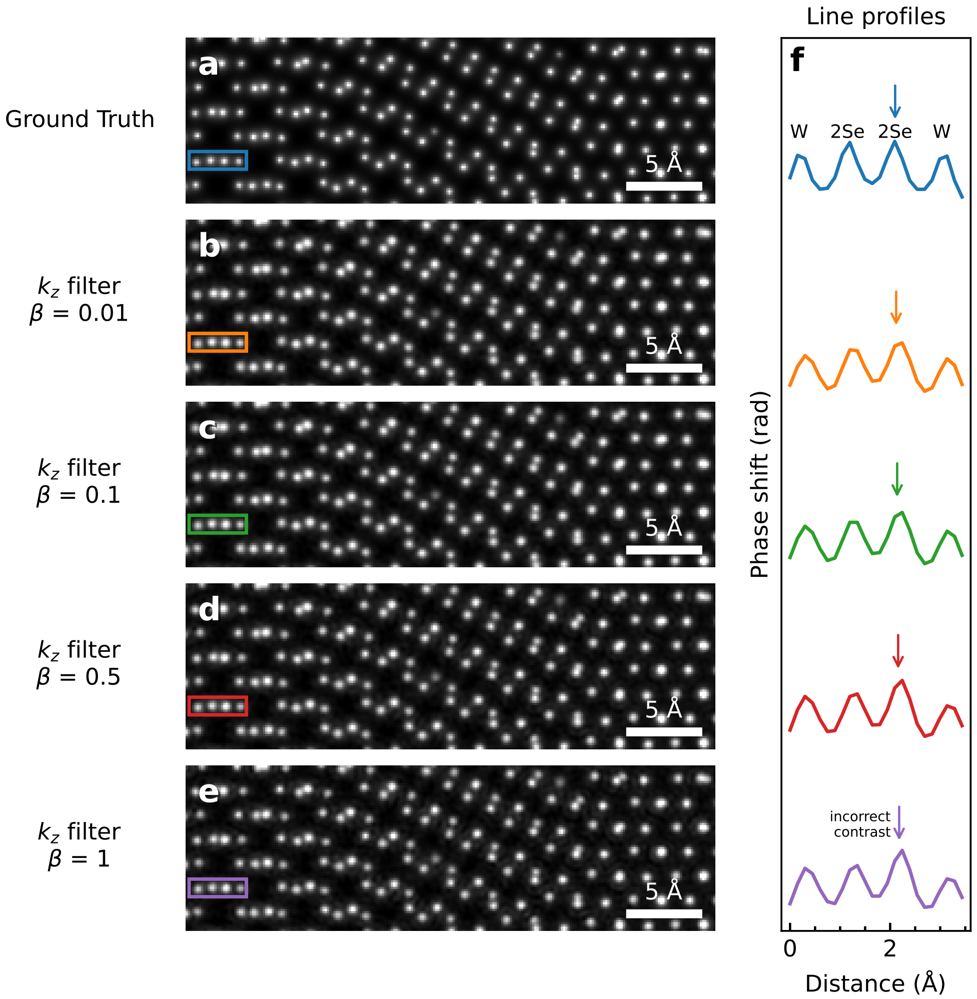


Supplementary Figure S8: Effect of $k_z$ regularization on ptychographic reconstruction of simulated tBL-$WSe_2$ using PtychoShelves. (a) Ground truth atomic potential. (b–e) Reconstructed phase images with increasing $k_z$ regularization parameters $\beta$ of 0.01, 0.1, 0.5, and 1, respectively. (f) Line profiles extracted from the marked regions in (a–e), corresponding to the W-2Se-2Se-W atomic columns. The arrows indicate the 2Se atomic site for each $k_z$ regularization value. As regularization increases, the local phase contrast becomes less accurate, highlighting the importance of selecting proper regularization parameters. 2Se corresponds to the atomic column with 2 overlapping Se atoms.

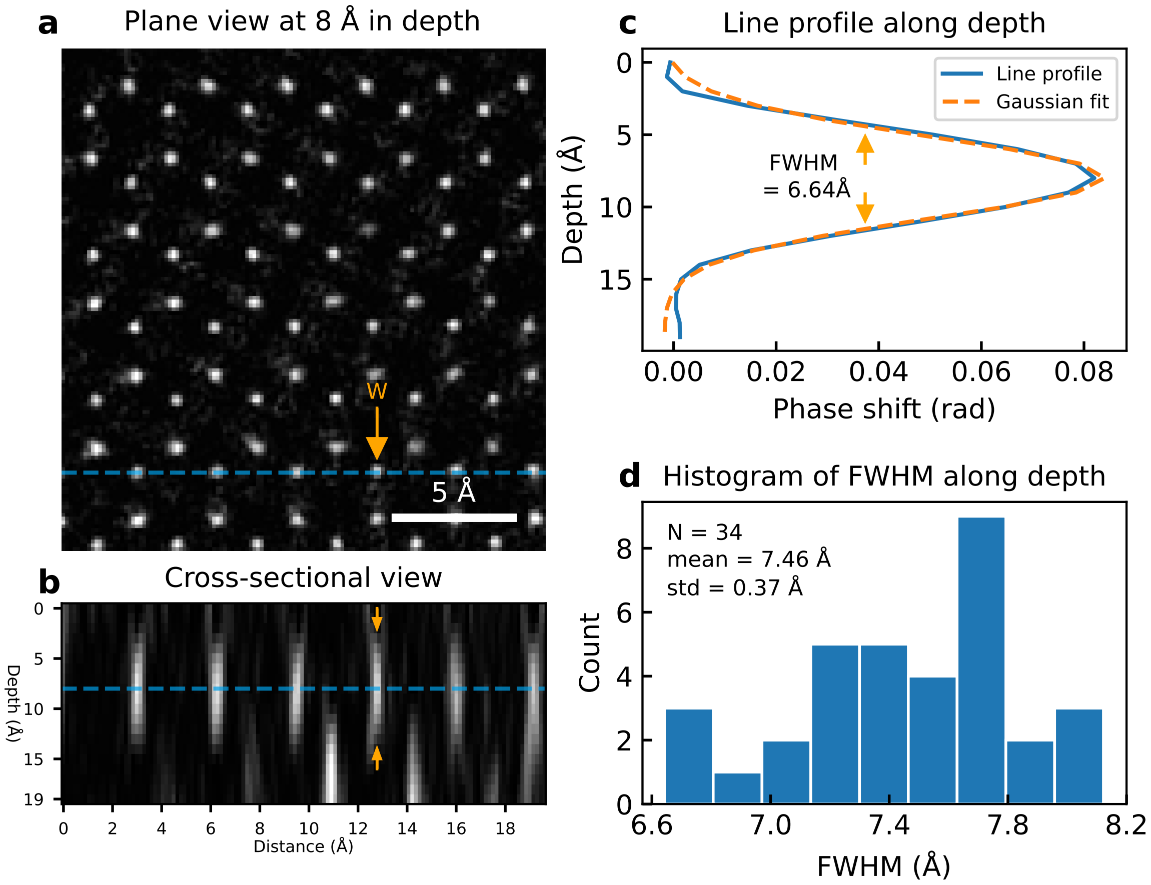


Supplementary Figure S9: Depth resolution analysis of multislice electron ptychography (MEP) reconstruction using the experimental tBL-$WSe_2$ dataset. The reconstruction was performed using PtyRAD with 12 probe modes, 20 object slices spaced by 1 Å, a batch size of 16, and regularization strategies including a positivity constraint, sparsity weight of 0.1, and an $r_z$ filter with $\sigma_z = 1$, over 1000 iterations. (a) Phase slice at 8 Å depth from the reconstructed 3D object stack, showing a top-down view of the top $WSe_2$ layer. The blue dashed line highlights a row of isolated W atoms used for depth analysis. (b) Cross-sectional view along the dashed line in (a), visualizing the reconstructed depth structure. The W atoms are vertically elongated due to the limited depth resolution of MEP. (c) Depth profile of a single W atom at the location marked by orange arrows in (a) and (b), with a Gaussian fit yielding a full width at half maximum (FWHM) of 6.64 Å. (d) Histogram of fitted FWHM values from 34 W atoms across the field-of-view (FOV) in (a), resulting a mean depth resolution of 7.46 Å with a standard deviation of 0.37 Å.

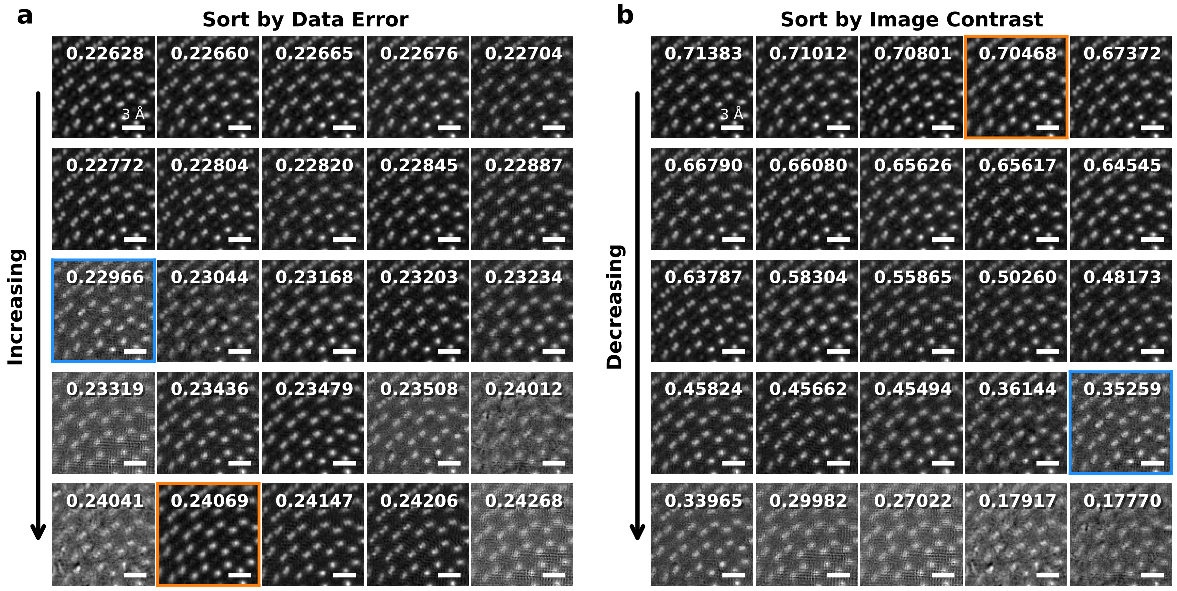


Supplementary Figure S10: Comparison of different error metrics for hyperparameter optimization. Collection of 25 reconstructed phase images sorted by (a) data error calculated with diffraction patterns in reciprocal space, and (b) image contrast calculated with the phase image. The images in (a) reveal a weak correlation between visual reconstruction quality and data error, indicating that lower data error does not consistently correspond to better visual quality. The blue box marks a low quality image with low data error, while the orange box marks a high quality reconstruction with higher data error. In contrast, the two images are sorted correctly with image contrast, and (b) shows a much stronger association between image contrast and perceived quality, suggesting that image contrast may serve as a more reliable metric for evaluating reconstruction quality, and hence more suitable for hyperparameter optimization.

# References


(1) Savitzky, B. H. et al. py4DSTEM: A Software Package for Four-Dimensional Scanning Transmission Electron Microscopy Data Analysis. Microscopy and Microanalysis **2021**, 27, 712–743.

(2) Jiang, Y. fold slice. https://github.com/yijiang1/fold_slice, 2020; https://github.com/yijiang1/fold_slice.

(3) Pennycook, T. J.; Lupini, A. R.; Yang, H.; Murfitt, M. F.; Jones, L.; Nellist, P. D. Efficient phase contrast imaging in STEM using a pixelated detector. Part 1: Experimental demonstration at atomic resolution. Ultramicroscopy **2015**, 151, 160–167.

(4) Yang, H.; Pennycook, T. J.; Nellist, P. D. Efficient phase contrast imaging in STEM using a pixelated detector. Part II: Optimisation of imaging conditions. Ultramicroscopy **2015**, 151, 232–239.

(5) Yang, H.; Rutte, R.; Jones, L.; Simson, M.; Sagawa, R.; Ryll, H.; Huth, M.; Pennycook, T.; Green, M.; Soltau, H.; others Simultaneous atomic-resolution electron ptychography and Z-contrast imaging of light and heavy elements in complex nanostructures. Nature Communications **2016**, 7, 12532.

(6) Enders, B.; Thibault, P. A computational framework for ptychographic reconstructions. Proceedings of the Royal Society A: Mathematical, Physical and Engineering Sciences **2016**, 472, 20160640.

(7) Dong, Z.; Fang, Y.-L. L.; Huang, X.; Yan, H.; Ha, S.; Xu, W.; Chu, Y. S.; Campbell, S. I.; Lin, M. High-performance multi-mode ptychography reconstruction on distributed GPUs. 2018 New York Scientific Data Summit (NYSDS). 2018; pp 1–5.

(8) Kandel, S.; Maddali, S.; Allain, M.; Hruszkewycz, S. O.; Jacobsen, C.; Nashed, Y. S. Us-

ing automatic differentiation as a general framework for ptychographic reconstruction. Optics express **2019**, 27, 18653–18672.

(9) Wakonig, K.; Stadler, H.-C.; Odstrčil, M.; Tsai, E. H. R.; Diaz, A.; Holler, M.; Usov, I.; Raabe, J.; Menzel, A.; Guizar-Sicairos, M. *PtychoShelves*, a versatile high-level framework for high-performance analysis of ptychographic data. Journal of Applied Crystallography **2020**, 53, 574–586.

(10) Favre-Nicolin, V.; Girard, G.; Leake, S.; Carnis, J.; Chushkin, Y.; Kieffer, J.; Paleo, P.; Richard, M.-I. PyNX: high-performance computing toolkit for coherent X-ray imaging based on operators. Journal of Applied Crystallography **2020**, 53, 1404–1413.

(11) Madsen, J.; Susi, T. The abTEM code: transmission electron microscopy from first principles. Open Research Europe **2021**, 1, 24.

(12) Cherukara, M. J.; Zhou, T.; Nashed, Y.; Enfedaque, P.; Hexemer, A.; Harder, R. J.; Holt, M. V. AI-enabled high-resolution scanning coherent diffraction imaging. Applied Physics Letters **2020**, 117.

(13) Yue, K.; Deng, J.; Jiang, Y.; Nashed, Y.; Vine, D. Ptychopy: GPU framework for ptychographic data analysis.

(14) Weber, D.; Lesnichaia, A.; Strauch, A.; Clausen, A.; Bangun, A.; Melnyk, O.; Meissner, H.; Ehrig, S.; Wendt, R.; Sukumaran, M.; et al. Ptychography 4.0: 0.1.0. https://zenodo.org/records/5055127.

(15) Du, M.; Kandel, S.; Deng, J.; Huang, X.; Demortiere, A.; Nguyen, T. T.; Tucoulou, R.; De Andrade, V.; Jin, Q.; Jacobsen, C. Adorym: A multi-platform generic X-ray image reconstruction framework based on automatic differentiation. Optics express **2021**, 29, 10000–10035.

(16) Seifert, J.; Bouchet, D.; Loetgering, L.; Mosk, A. P. Efficient and flexible approach to ptychography using an optimization framework based on automatic differentiation. OSA Continuum **2021**, 4, 121–128.

(17) Gursoy, D.; Ching, D. J. Tike; 2022.

(18) Guzzi, F.; Kourousias, G.; Billè, F.; Pugliese, R.; Gianoncelli, A.; Carrato, S. A modular software framework for the design and implementation of ptychography algorithms. PeerJ Computer Science **2022**, 8, e1036.

(19) Friedrich, T.; Yu, C.; Verbeeck, J.; Van Aert, S. Phase Object Reconstruction for 4D-STEM using Deep Learning,(4D-STEM Example Data). URL https://doi.org/10.5281/zenodo **2022**, 7034879.

(20) Chang, D. J.; O'Leary, C. M.; Su, C.; Jacobs, D. A.; Kahn, S.; Zettl, A.; Ciston, J.; Ercius, P.; Miao, J. Deep-learning electron diffractive imaging. Physical review letters **2023**, 130, 016101.

(21) Loetgering, L.; Du, M.; Boonzajer Flaes, D.; Aidukas, T.; Wechsler, F.; Penagos Molina, D. S.; Rose, M.; Pelekanidis, A.; Eschen, W.; Hess, J.; others PtyLab. m/py/jl: a cross-platform, open-source inverse modeling toolbox for conventional and Fourier ptychography. Optics Express **2023**, 31, 13763–13797.

(22) Diederichs, B.; Herdegen, Z.; Strauch, A.; Filbir, F.; Müller-Caspary, K. Exact inversion of partially coherent dynamical electron scattering for picometric structure retrieval. Nature Communications **2024**, 15, 101.

(23) Nakahata, R.; Zaman, S.; Zhang, M.; Lu, F.; Chiu, K. PtychoFormer: A Transformer-based Model for Ptychographic Phase Retrieval. arXiv preprint arXiv:2410.17377 **2024**,

(24) Zhang, H.; Li, G.; Zhang, J.; Zhang, D.; Chen, Z.; Liu, X.; Guo, P.; Zhu, Y.; Chen, C.;

Liu, L.; Guo, X.; Han, Y. Three-Dimensional Inhomogeneity of Zeolite Structure and Composition Revealed by Electron Ptychography. Science **2023**, 380, 633–638.

(25) Li, G.; Xu, M.; Tang, W.-Q.; Liu, Y.; Chen, C.; Zhang, D.; Liu, L.; Ning, S.; Zhang, H.; Gu, Z.-Y.; Lai, Z.; Muller, D. A.; Han, Y. Atomically Resolved Imaging of Radiation-Sensitive Metal-Organic Frameworks via Electron Ptychography. Nature Communications **2025**, 16, 914.

(26) Nguyen, K. X.; Jiang, Y.; Lee, C.-H.; Kharel, P.; Zhang, Y.; van der Zande, A. M.; Huang, P. Y. Achieving sub-0.5-angstrom–resolution ptychography in an uncorrected electron microscope. Science **2024**, 383, 865–870.

(27) Chen, Z.; Jiang, Y.; Shao, Y.-T.; Holtz, M. E.; Odstrčil, M.; Guizar-Sicairos, M.; Hanke, I.; Ganschow, S.; Schlom, D. G.; Muller, D. A. Electron ptychography achieves atomic-resolution limits set by lattice vibrations. Science **2021**, 372, 826–831.
